# Supplementary material for: Graph Component Contrastive Learning for Concept Relatedness Estimation
Source: arXiv:2206.12556 source file (2022-11-30)
Supplement: Supplementary file 1 [file appendix.tex]

\section{Model Configurations}

Model specification for the transformer models.

\begin{table}[htb]
\begin{center}
% \vspace{3mm}
\begin{tabular}{l l}
\toprule
  Hidden Activation   & GELU \\
 \hline
  Dropout Probability & 0.1 \\
 \hline
  Hidden Size         & 768 \\
 \hline
  Intermediate Size   & 3072 \\
 \hline
  Max Position Embeddings & 512 \\
 \hline
  Num Attention Heads & 12 \\
 \hline
  Num Hidden Layers   & 12 \\
 \hline
  Vocab Size          & \thead{30522 (EN)\\21128 (CN)} \\
\bottomrule
\end{tabular}
\caption{ConcreteBERT architecture details (BERT base)}
\label{tb:BERT_config}
\end{center}
\end{table}

% \begin{table}[h]
% \begin{center}
% \caption{ConcreteBERT architecture details for the CNSE dataset and the CNSS dataset}
% % \vspace{3mm}
% \begin{tabular}{l l}
% \toprule
%   Hidden Activation   & GELU \\
%  \hline
%   Dropout Probability & 0.1 \\
%  \hline
%   Hidden Size         & 768 \\
%  \hline
%   Intermediate Size   & 3072 \\
%  \hline
%   Max Position Embeddings & 512 \\
%  \hline
%   Num Attention Heads & 12 \\
%  \hline
%   Num Hidden Layers   & 12 \\
%  \hline
%   Vocab Size          & 21128 \\
% \bottomrule
% \end{tabular}
% \label{tb:BERT_config_chinese}
% \end{center}
% \end{table}

\begin{table}[htb]
\begin{center}
% \vspace{3mm}
\begin{tabular}{l l}
\toprule
  Hidden Activation   & GELU \\
 \hline
  Dropout Probability & 0.1 \\
 \hline
  Hidden Size         & 768 \\
 \hline
  Intermediate Size   & 3072 \\
 \hline
  Max Position Embeddings & 514 \\
 \hline
  Num Attention Heads & 12 \\
 \hline
  Num Hidden Layers   & 12 \\
 \hline
  Vocab Size          & \thead{50265 (EN)\\21128 (CN)} \\
\bottomrule
\end{tabular}
\caption{RoBERTa architecture details (RoBERTa base)}
\label{tb:RoBERTa_config}
\end{center}
\end{table}

\begin{table}[htb]
\begin{center}
% \vspace{3mm}
\begin{tabular}{l l}
\toprule
  Hidden Activation   & GELU \\
 \hline
  Dropout Probability & 0.1 \\
 \hline
  Hidden Size         & 768 \\
 \hline
  Intermediate Size   & 3072 \\
 \hline
  Num Attention Heads & 12 \\
 \hline
  Num Hidden Layers   & 12 \\
 \hline
  Attention Head Size & 64 \\
 \hline
  Vocab Size          & \thead{32000 (EN)\\32000 (CN)}\\
\bottomrule
\end{tabular}
\caption{XLNet architecture details (XLNet base)}
\label{tb:XLNet_config}
\end{center}
\end{table}

\section{Metrics}

\begin{equation}
\begin{split}
\text{precision} &= \frac{TP}{TP + FP},\\
\text{recall} = \text{sensitivity} &= \frac{TP}{TP + FN},\\
\text{specificity} &= \frac{TN}{TN + FP},\\
\text{F1 score} & = \frac{2}{\text{precision}^{-1} + \text{recall}^{-1}},
\end{split}
\label{eq:metrics}
\end{equation}
where TP = true positives, FP = false positives, TN = true negatives, FN = false negatives.

\section{Dataset Statistics}
\begin{table}[H]
\begin{center}
\resizebox{0.9\columnwidth}{!}{
\begin{tabular}{l l l l}
\toprule
     & WORD & CNSE & CNSS \\
 \hline
 Total Size      & 19,176 &  29,063 &  33,503 \\
 Positive Count  & 10,028 & 12,865 & 16,887 \\
 Negative Count  & 9,148 & 16,198 & 16,616 \\
 \hline
 Training Size   & 11,563 & 20,342 & 23,449 \\
 Validation Size & 1,287 & 5,812 & 6,700 \\
 Test Size       & 6,302 & 2,907 & 3,351 \\
\bottomrule
\end{tabular}}
\caption{Statistics of the WORD dataset, the CNSE dataset and the CNSS dataset}
\label{tb:Dataset_statistics}
\end{center}
\end{table}

\section{T-Tests}
\label{sec:t-tests}
We conduct t-tests assuming unequal variances. The improvement from our method is statistically significant when the p-value is less than 5\%. We ran XLNet \cite{DBLP:conf/nips/YangDYCSL19} five additional times on CNSS \cite{DBLP:conf/acl/LiuNWGHLX19}, and t-tests against the base Transformer model show that GCCL is statistically significant (one-tail p-value $< 0.05$):
\begin{table}[H]
\begin{center}
\resizebox{0.9\columnwidth}{!}{
\begin{tabular}{l l l l}
\toprule
     & XLNet & GCCL & GCCL+Aug \\
 \hline
 Acc & 91.24$\pm$1.87  & 93.18$\pm$0.49 & 92.93$\pm$0.46 \\
 P-value  & - & 0.0089 & 0.0152 \\
 \hline
 F1 & 91.13$\pm$2.40  & 93.35$\pm$0.47 & 93.23$\pm$0.38 \\
 P-value  & - & 0.0075 & 0.0088 \\
 \hline
 Auc & 97.75$\pm$0.18  & 98.39$\pm$0.05 & 98.18$\pm$0.06 \\
 P-value  & - & 0.0057 & 0.0334 \\
\bottomrule
\end{tabular}}
\caption{Statistics of the WORD dataset, the CNSE dataset and the CNSS dataset}
\label{tb:t-tests}
\end{center}
\end{table}

\section{Traditional Algorithms}
\label{sec:trad_algo}

We include two traditional algorithms, BM25 \cite{DBLP:journals/ftir/RobertsonZ09} and LDA \cite{blei2003latent}. In the BM25-based relatedness estimation algorithm (Appendix: Algorithm~\ref{algo:bm25}), we use BM25 to query the source concept in the dataset and check whether the target concept is a match, which means they are a related concept pair. In the LDA-based relatedness estimation algorithm (Appendix: Algorithm~\ref{algo:lda}), we first train the LDA model to learn what topics exist in the dataset; then we obtain the topic distributions of concept pairs with the trained LDA model and calculate the cosine similarity between their topic distributions, which estimates the relatedness.

\begin{table}[h]
  \centering
  \resizebox{1\columnwidth}{!}{\begin{tabular}{l|c c |c c |c c }
    \toprule
        & \multicolumn{2}{c|}{\textbf{WORD}}  & \multicolumn{2}{c|}{\textbf{CNSE}}  & \multicolumn{2}{c}{\textbf{CNSS}}  \\ 
    Model & Acc & F1 & Acc & F1 & Acc & F1 \\ 

    \Xhline{2\arrayrulewidth}

    LDA & 49.94 & 48.44 & 57.74 & 43.54 & 51.89 & 61.40 \\
    BM25 & 51.87 & 41.31 & 69.56 & 70.25 & 66.25 & 63.60 \\
    \bottomrule
  \end{tabular}
  }
  \caption{Performance of LDA and BM25.}
%   \label{tb:performance_comp}
\end{table}

\newpage

The pseudo-code for baselines, LDA and BM25.

\begin{algorithm}[H]
\caption{BM25-based relatedness estimation}
\label{algo:bm25}
% \begin{multicols}{2}
\begin{algorithmic}[1]
% \DontPrintSemicolon
\Require{testPairs \{($A_{1}$, $B_{1}$, $score_1$), ($A_{2}$, $B_{2}$, $score_2$), ($A_{3}$, $B_{3}$, $score_3$) \dots, ($A_{n}$, $B_{n}$, $score_n$)\}, threshold T}
\Ensure{testAccuracy}
\State $score = \{\}$
% \Comment{use dictionary $score$ to store the similarity score of every pair of documents}
\State $Documents = [A_1, B_1, A_2, B_2, \dots, A_n, B_n]$
\State $testNum = 0$
\State $predictTrue = 0$

\For{every pair ($A_i$, $B_i$, $score_i$) in testPairs}
\State $q = A_i$
\State $score[A_i] = []$
\For{every d in Documents}
    \State $newScore = BM25(d, q)$
    \State $score[A_i].append(newScore)$
    \State $testNum += 1$
\EndFor
\State $q = B_i$
\State $score[B_i] = []$
\For{every d in Documents}
\State $newScore = BM25(d, q)$
\State $score[B_i].append(newScore)$
\State $testNum += 1$
\EndFor
\State $Normalize(score[A_i])$
\State $Normalize(score[B_i])$
\If{$score_i > 0$}
    \If{$score[A_i][2i-1] > T $}
        \State $predictTrue +=1$
    \EndIf
    \If{$score[B_i][2(i-1)] > T $}
        \State $predictTrue +=1$
    \EndIf
\Else
    \If{$score[A_i][2i-1] < T $}
        \State $predictTrue +=1$
    \EndIf
    \If{$score[B_i][2(i-1)] < T $}
        \State $predictTrue +=1$
    \EndIf
\EndIf
\EndFor
\State $testAccuracy = predictTrue / testNum$\;
\Return testAccuracy
\end{algorithmic}
% \end{multicols}
\end{algorithm}

To calculate the score for a document, we use the following function based on BM25:
\begin{equation}
\begin{split}
& BM25(d, q)= \sum_{i}log\frac{N-n(q_i)+0.5}{n(q_i)+0.5}\cdot\\
& \frac{(k_1+1)\cdot tf(q_i, d)}{k_1(1-b+b\cdot \frac{L_d}{L_{avg}})+tf(q_i, d)}\cdot \frac{(k_2+1)\cdot tf(q_i, q)}{k_2+tf(q_i, q)}
\end{split}
\end{equation}
where $N$ is the total number of Documents, $q_i$ is the i-th token in document $q$, $n(q_i)$ is the number of documents contains token $q_i$, $k_1, k_2, b$ are three parameters, $tf(a, b)$ is the frequency of token $a$ in $b$, $L_d$ is the length of document $d$ and $L_{avg}$ is the average length of all documents.

\begin{algorithm}[H]
\caption{LDA based relatedness estimation}
\label{algo:lda}
\begin{algorithmic}[1]
% \DontPrintSemicolon
\Require{trainPairs \{($A_{1}$, $B_{1}$), ($A_{2}$, $B_{2}$), ($A_{3}$, $B_{3}$) \dots, testPairs \{($C_{1}$, $D_{1}$, $score_1$), ($C_{2}$, $D_{2}$, $score_2$), ($C_{3}$, $D_{3}$) \dots, ($C_{n}$, $D_{n}$)\}, threshold T}
\Ensure{testAccuracy}

\Comment{First, we clean and tokenize the text in trainPairs and testPairs}
\State $trainDf = [A^t_1, B^t_1, A^t_2, B^t_2, \dots, A^t_n, B^t_n]$
\State $testDf = [(C^t_1, D^t_1, score_1), $
    $(C^t_2, D^t_2, score_2), \dots, (C^t_n, D^t_n, score_n)]$
\State $ldaModel = trainLda(trainDf)$
\State $testNum = 0$
\State $predictTrue = 0$
\For{every pair ($C^t_i, D^t_i, score_i$) in testDf}
\Comment{We can obtain the topic distribution with the model trained on docs from trainPairs}
\State $\textbf{distributionC} = ldaModel(C^t_i)$
\State $\textbf{distributionD} = ldaModel(D^t_i)$
\Comment{We use the cosine similarity of the two topic distribution for the related estimation for the doc pair}
\State $similarity = \frac{\textbf{distributionC} \cdot
\textbf{distributionD}}{||\textbf{distributionC}||\cdot||\textbf{distributionD}||}$
\State $testNum +=1$

\If{$score_i > 0$}
    \If{$similarity >= T$}
    \State $predictTrue +=1$
    \EndIf
\Else
    \If{$similarity < T$}
    \State $predictTrue +=1$
    \EndIf
\EndIf
\EndFor
\State $testAccuracy = predictTrue / testNum$\;
\Return testAccuracy
\end{algorithmic}
\end{algorithm}

In our implementation, $T=0.004$.
